# Supplementary material for: Topics in the phenomenology of axions: the cases of cosmic strings and superradiance
Source: arXiv:2608.23789 source file (2026-08-24)
Supplement: Supplementary file 1 [file appendix.tex]

\chapter{Density correlations in expanding universe}
\label{app:density correl}
We list here the correlation functions of the scalar field $\phi$ that are need to calculate the density correlations $\langle \rho(x) \rho(x') \rangle$:
\begin{align}
       & \langle \phi(x) \phi(x') \rangle  = \int \frac{d^{3}k}{(2 \pi)^{3}} F_{k} \cos \left[ \int^{t}_{t'} dt'' \omega_{k}(t'') - \textbf{k} \cdot \Delta \textbf{k} \right] \\  &
        \langle \dot{\phi}(x) \phi(x') \rangle = - \int \frac{d^{3}k}{(2 \pi)^{3}} F_{k} \omega_{\bf k}(t) \sin \left[ \int^{t}_{t'} dt'' \omega_{k}(t'') - \textbf{k} \cdot \Delta \textbf{k} \right] \\  &
        \langle \phi(x) \nabla \phi(x') \rangle = - \int \frac{d^{3}k}{(2 \pi)^{3}} F_{k} \textbf{k} \sin \left[ \int^{t}_{t'} dt'' \omega_{k}(t'') - \textbf{k} \cdot \Delta \textbf{k} \right]  \\  &
        \langle \dot{\phi}(x) \dot{\phi}(x') \rangle = \int \frac{d^{3}k}{(2 \pi)^{3}} F_{k} \omega_{\bf k}(t) \omega_{\bf k}(t') \cos \left[ \int^{t}_{t'} dt'' \omega_{k}(t'') - \textbf{k} \cdot \Delta \textbf{k} \right] \\ &
           \langle \dot{\phi}(x) \nabla\phi(x') \rangle = -\int \frac{d^{3}k}{(2 \pi)^{3}} F_{k} \omega_{\bf k}(t) \textbf{k} \cos \left[ \int^{t}_{t'} dt'' \omega_{k}(t'') - \textbf{k} \cdot \Delta \textbf{k} \right] \\ &
           \langle \partial_{i}\phi(x) \partial_{j}\phi(x') \rangle = \int \frac{d^{3}k}{(2 \pi)^{3}} F_{k} k_{i} k_{j} \cos \left[ \int^{t}_{t'} dt'' \omega_{k}(t'') - \textbf{k} \cdot \Delta \textbf{k} \right] 
\end{align}
where $F_{k}$ is defined as:

\begin{equation}
    F_k(t,t') \equiv \frac{f(k)}{\sqrt{a^{3}(t) \omega_{\textbf{k}}(t) a^{3}(t') \omega_{\textbf{k}}(t')}}
\end{equation}

It is straightforward to use these field correlators to find the density correlations $\langle \rho(x) \rho(x') \rangle$. As discussed, these split into terms $\langle \rho(x) \rho(x') \rangle = \langle \rho(x) \rho(x') \rangle_{+} + \langle \rho(x) \rho(x') \rangle_{-}$, which have the general form:
\begin{align}
\label{eqn:correlations density}
\begin{split}
    &\langle \rho(x) \rho(x') \rangle_{\pm} = \frac{1}{4} \int \frac{d^{3}k d^{3}k'}{(2 \pi)^{6}}  F_{k} F_{k'} A^{\pm}_{\bf k k'} \times  \\ & \times \cos \left[ \int^{t}_{t'} dt'' (\omega_{\bf k}(t'') \pm \omega_{\bf k'}(t'')) - (\textbf{k} \pm \textbf{k}') \cdot \Delta\textbf{x} \right]
\end{split}
\end{align}
with the coefficients $A^{\pm}_{\bf k k'}$ given explicitly by: 
\begin{align}
    \begin{split}
        A^{\pm}_{\bf k k'}  = 
         & m^{2}(t) m^{2}(t')+\omega_{\bf k}(t) \omega_{\bf k}(t') \omega_{\bf k'}(t) \omega_{\bf k'}(t') \mp  m^{2}(t')\omega_{\bf k}(t) \omega_{\bf k'}(t) \mp m^{2}(t) \omega_{\bf k}(t') \omega_{\bf k'}(t') +  \\ & + \textbf{k} \cdot \textbf{k}' \left( \frac{\omega_{\textbf{k}}(t) \omega_{\textbf{k}'}(t) \mp m^{2}(t)}{a^{2}(t')} + \frac{\omega_{\textbf{k}}(t') \omega_{\textbf{k}'}(t') \mp m^{2}(t')}{a^{2}(t)} \right) + \frac{\left( \textbf{k} \cdot \textbf{k}'\right)^{2}}{a^{2}(t) a^{2}(t')}
         \end{split}
\end{align}
In the non-relativistic limit where $\omega_{\bf k}(t) \simeq m(t) + \textbf{k}^{2}/2 m a^{2}(t)$, these coefficients become $A^{+}_{\bf k k'} \simeq \left( |\textbf{k} + \textbf{k}'|^{2}  \right)^{2}/4 a^{2}(t) a^{2}(t')$ and $A^{-}_{\bf k k'} \simeq 4 m^{2}(t) m^{2}(t')$.

\chapter{The Maxwell-Boltzmann distribution}
\label{sec:maxwell}

It is illuminating to compare the cosmic string spectrum to that of the familiar Maxwell-Boltzmann distribution. To that end, we briefly summarize the results in this case. We assume that the particles start to behave non-relativistically at time $t_{m}$, with corresponding scale factor $a_{m}$, and that their phase space distribution evolves self-similarly after that. We evaluate \Eq{eqn:correlations density} at $t=t'=t_{m}$.  We may first write the integrals and the phase space densities in terms of the velocity $v$:
\begin{align}
\begin{split}
   & f\left( k \right)  \frac{d^{3} k}{a^{3}_{m} (2\pi)^{3}}=  \frac{\bar{\rho}(t_{m})}{m} f\left( v \right) d^{3} v.
\end{split}
\end{align}
We have defined $f(v)$ in such a way that $\int d^{3}v f(v) = 1$.
Plugging this in \Eq{eqn:correlations density} and focusing on the slow mode, we get:
\begin{align}
\begin{split}
     &\langle \rho_{\phi}(\textbf{x}) \rho_{\phi}(\textbf{x}') \rangle_{-} \\&=  \bar{\rho}^{2}(t_{m})  \int   d^{3}v d^{3}v'  f(v) f(v') 
    \cos \left( m\Delta \textbf{x} \cdot \Delta \bf{v} \right),
\end{split}
\label{eqn:rho correl approx}\end{align}
where we defined $\Delta \textbf{v} = \textbf{v} - \textbf{v}'$.

The Maxwell-Boltzmann distribution is given by $f(v) =  e^{-v^{2}/2 v^{2}_{0} a^{2}_{m}}/(2 \pi v^{2}_{0} a^{2}_{m})^{3/2}$. Plugging this in \Eq{eqn:rho correl approx} and employing the transformations $\textbf{v}_{\pm} = (\textbf{v} \pm \textbf{v}')/\sqrt{2}$ to simplify the integrals, we get: 

\begin{align}
\begin{split}
     \langle \rho_{\phi}(\textbf{x}) \rho_{\phi}(\textbf{x}') \rangle_{-} =  & \frac{\bar{\rho}^{2}_{\phi}(t_{m})}{\left( 2\pi v^{2}_{0} a^{2}_{m} \right)^{3}}  \int d^{3}v_{+} d^{3}v_{-} e^{- \frac{v_{+}^{2} + v_{-}^{2}}{2 v^{2}_{0} a^{2}_{m}}} 
   \\ & 
    \cos \left( \sqrt{2} \Delta \textbf{x} \cdot \textbf{v}_{-} \right),
\end{split}
\label{eqn:rho correl v+}
\end{align}
These integrals can be done analytically and we obtain:
\begin{equation}
     \langle \rho_{\phi}(\textbf{x}) \rho_{\phi}(\textbf{x}') \rangle_{-} =  \bar{\rho}_{\phi}^{2}(t_{m}) e^{  - k^{2}_\star \Delta \textbf{x}^{2}},
\label{eqn:density correl space}
\end{equation}
where $k_\star = a_{m} m v_{0}$.
The power spectrum is then:
\begin{align}
\begin{split}
    P_{\phi}(k,t_{m}) \equiv  &  \int d^{3} x e^{-i \textbf{k} \cdot \textbf{x}}  \frac{\langle \rho_{\phi}(\textbf{x}) \rho_{\phi}(0) \rangle}{\bar{\rho}^{2}_{\rm DM}(t_{m})}  = \\ & = \left( \frac{\bar{\rho}_{\phi}(t_{0})}{\bar{\rho}_{\rm DM}(t_{0})} \right)^{2} \pi^{3/2} \left( \frac{1}{k_\star} \right)^{3} \mathcal{T}_{\rm MB} \left( \frac{k}{k_\star}\right),
\end{split}
\label{eqn:uldm power spectrum}
\end{align}
where we considered that the dark matter as well as the ultra light axion's density both scale as $a^{-3}$ and defined the transfer function $\mathcal{T}_{\rm MB}(y) = e^{-y^{2}/4}$. This is the transfer function that we depict in \Fig{fig:transfer functions}. 

\chapter{Infrared cut-off of spectrum}
\label{section:Cut-off}

The infrared cutoff that was given in \cref{eqn:kir}, may depend on $f_{a}$ if $n \neq 0$. Parametrically, we have for $a_{m}$:

\begin{equation}
    a_{m} \propto \frac{a_{\rm eq} T_{\rm eq}}{\sqrt{m_{a,0} M_{\rm pl}}} \left( \frac{M_{\rm pl}}{f_{a}} \right)^{\frac{n}{2n+4}}
\end{equation}

where we used the definition of $a_{m}$ through $H(a_{m}) = m(a_{m})$ and:

\begin{equation}
    H(a_{m}) \propto \frac{T^{2}_{\rm eq} a^{2}_{\rm eq}}{M_{\rm pl} a^{2}_{m}}
\end{equation}


where $T_{\rm eq} \simeq 0.1 \rm eV$ is the temperature at the time of the radiation-matter equality. The infrared cutoff then scales as:
\begin{equation}
k_{\rm IR} \propto a_{\rm eq} T_{\rm eq} \sqrt{\frac{m_{a,0}}{M_{\rm pl}}} \left( \frac{f_{a}}{M_{\rm pl}}\right)^{\frac{n}{2n+4}} x_{\rm IR}
\end{equation}

Therefore, for the same mass and $x_{\rm IR}$, the effect of temperature dependence is to shift the infrared cut-off to smaller energies, in the physically relevant regime $f_{a} < M_{\rm pl}$. 


\chapter{Free-streaming}
\label{sec:free streaming}
To determine the free-streaming constraint, we follow \cite{amin2024lowerbounddarkmatter,Liu:2024pjg,Long:2024cak}. The free streaming length is given by \Eq{eqn:free streaming scale}. 
This integral can be determined analytically for any scale factor and momentum $k$, in the case where the mass is temperature independent, and the result is (see appendix A of \cite{Liu:2024pjg}):

\begin{equation}
    \lambda_{\rm fs}(k,a) = \frac{\sqrt{2}}{H_{\rm eq} a_{\rm eq}} F\left(\hat{k},y\right)
\end{equation}

where $\hat{k} \equiv k/m a_{\rm eq}$, $y \equiv a/a_{\rm eq}$ and $F(\hat{k},y)$ is a function that is given in the appendix A of \cite{Liu:2024pjg}. For non-relativistic momenta at equality, $\hat{k} \ll 1$, the dominant contribution to the free-streaming length comes from $y \ll 1$ and it is logarithmic in $y$. For temperature dependent masses, the integral can be performed numerically.

As it was shown in \cite{amin2024lowerbounddarkmatter}, free streaming affects only the adiabatic part of the power spectrum and it is encoded in the transfer function:

\begin{equation}
\label{eqn:transfer fs}
    T_{\rm fs}(k,a) = \frac{m^{2}_{\rm NR}}{\bar{\rho}_{\rm DM}(a)}\int \frac{d^{3} p}{(2 \pi)^{3}}\mathcal{P}(p) \sinc \left( p \lambda(p,a) \right)
\end{equation}

where $\mathcal{P}(p)$ is an initial power spectrum of fluctuations. This is related to the usual phase space density through \cite{Long:2024cak}:

\begin{equation}
\label{eqn:P to f}
    f(p,t) = a^{3}(t) \omega_{\textbf{p}}(t) \mathcal{P}(p)
\end{equation}

Relating this phase space density to our spectrum $\Omega_{\phi}$ through \Eq{eqn:f and Omega} and plugging it in \Eq{eqn:transfer fs}, we obtain:

\begin{equation}
    T_{\rm fs}(k,a) = \frac{m_{\rm NR} \rho_{c}(a_{\rm NR}) a^{4}_{\rm NR}}{\bar{\rho}_{\rm DM}(a_{0}) } \int \frac{dp}{p^{2}} \Omega_{\phi}(p) \sinc \left( k \lambda(p,a) \right)
\end{equation}

In the case where the spectrum $\Omega_{\phi}(k)$ is dominated  at $k_\star$, the integral can be simplified to give \Eq{eqn:transfer free approx} where we also used \Eq{eqn:relic density}.
To draw the bound, we performed the integral in \Eq{eqn:transfer fs} numerically, evaluated at the present time, and used the spectrum given in \Eq{eqn:Omega}.



\chapter{Gravitational atom basics}
\section{Tidal Field of the Companion}
\label{appendix: tidal}
We present in this appendix some of the formulae we used for the tidal field of the companion and the Hamiltonian for the two state system.
The tidal field is given as a sum over multipoles:

\begin{equation}
    V_{\ast}(t,\vec{r}) = -q \alpha \sum_{l_{\ast} = 2} \sum_{|m_{\ast}|\leq l_{\ast}} \mathcal{E}_{l_{\ast},m_{\ast}}(\iota_{\ast},\varphi_{\ast}) Y_{l_{\ast},m_{\ast}}(\theta,\phi) \left(\frac{r^{l_{\ast}}}{R^{l_{\ast}+1}} \Theta(R_{\ast} - r) + \frac{R_{\ast}^{l_{\ast}}}{r^{l_{\ast}+1}} \Theta(r - R_{\ast})\right),
\end{equation}
where $R_{\ast}$ is the distance of the companion from the primary black hole, $\mathcal{E}_{l_{\ast},m_{\ast}} (\iota_{\ast},\varphi_{\ast})$ is the tidal moment (see Appendix A of \cite{Baumann_2020} for details), $\iota_{\ast}$ is the inclination of the orbital plane relative to the GA's, $\varphi_{\ast}$ is the true anomaly and is related to the frequency of the binary via $\dot{\varphi_*}(t) = \pm \Omega(t) $. We have also defined $q = \frac{M_{\ast}}{M}$ as the mass ratio.

Assuming that the quadrupole dominates, the mixing between two states $| \psi_{i} \rangle$ and $| \psi_{f} \rangle$ is given by
\begin{equation}
   \langle \psi_{f} |V_{\ast} (t,\vec{r}) | \psi_{i} \rangle  = \mathcal{E}_{2,m_{\ast}} (\iota_{\star},\varphi_{\ast}) I_{A} \left( \frac{ q M \Omega }{\alpha^{3} (1+q)} I_{\textrm{in}} + \frac{\alpha^{7} q (1+q)^{2/3}}{(M \Omega)^{7/3}} I_{\textrm{out}} \right),                            
\label{eqn:V}\end{equation}
where the inner radial, outer radial, and angular overlaps of the initial and final wavefunction mediated by the quadrupole moment of the tidal field are:
\begin{align}
    & I_{\textrm{in}}  = \int^{R_{\ast}/r_{c}}_{0} d \bar{r} \bar{r}^{4} \bar{R}_{i} (r_{c} \bar{r}) \bar{R}_{f} (r_{c} \bar{r}),  \\
    & I_{\textrm{out}} = \int^{\infty}_{R_{\ast}/r_{c}} d \bar{r} \bar{r}^{-1} \bar{R}_{i} (r_{c} \bar{r}) \bar{R}_{f} (r_{c} \bar{r}), \\
    & I_{A} = \int d \Omega Y_{l_{\ast},m_{\ast}} (\theta,\varphi) Y_{i}(\theta,\varphi) Y^{\ast}_{f}(\theta,\varphi), 
\end{align}
with new dimensionless quantities $\bar{r} = \frac{r}{r_{c}}$ and $\bar{R} (r_{c} \bar{r})=R(r)r^{3/2}_{c}$. The selection rules \Eq{eq:selection_rule} are derived from the last angular integral. Taking $\iota_{\ast} = 0$, the amplitude of the mixing normalized by the orbital frequency is:
\begin{equation}
    \frac{\eta}{\Omega}  = \left|\sqrt{\frac{3 \pi}{10}}  I_{A} \left( \frac{ q M \Omega }{\alpha^{3} (1+q)} I_{\textrm{in}} + \frac{\alpha^{7} q (1+q)^{2/3}}{(M \Omega)^{7/3}} I_{\textrm{out}} \right)\right|,
\label{eqn:eta}\end{equation}
and the matrix element is given in \Eq{eqn:matrix element}.


\section{Dressed Frame Hamiltonian}
\label{appendix:Hamiltonian}
\par
In the dressed co-rotating frame, the Hamiltonian is given by:
\begin{equation}
\bar{\mathcal{H}} = 
    \begin{pmatrix}
  - \frac{\Delta m}{2} (\frac{\Delta \omega_{R}}{\Delta m}  \mp\Omega(t))   &  \eta  \\
    \eta   &   \frac{\Delta m}{2} (\frac{\Delta \omega_{R}}{\Delta m} \mp \Omega(t) ) - i |\Gamma| 
\end{pmatrix}.
\label{eqn:dressed Hamiltonian}\end{equation}

Choosing $\Omega_{0} = \pm \frac{\Delta \omega_{R}}{\Delta m}$ and using \Eq{eqn:linear freq}, we obtain the Hamiltonian of the Landau-Zener system (for a co-rotating orbit),
\begin{equation}
\bar{\mathcal{H}} = 
    \begin{pmatrix}
   \frac{\Delta m}{2} \gamma t   &  \eta  \\
    \eta   &  - \frac{\Delta m}{2} \gamma t - i |\Gamma|
\end{pmatrix}.
\label{eqn:Hamiltonian}\end{equation}

The second order differential equations for $d_{1}(t)$ and $d_{2}(t)$ are
\begin{align}
   & d''_{i}(\tau) + d_{i}(\tau)\left( \frac{\tau^{2}}{4}  -  \frac{i}{2}  + z \right) = 0,  \\
   & d''_{f}(\tau) + d_{f}(\tau)\left( \frac{\tau^{2}}{4}  +  \frac{i}{2}  + z \right) = 0 , 
\label{eqn:equation of motion}\end{align}
where we have defined $\tau = \sqrt{|\Delta m| \gamma} t$ and set $\Gamma =0$. The prime denotes the derivative with respect to $\tau$. The solutions to these equations are given in \Eq{eq:coefficient_d1} and \Eq{eq:coefficient_d2} and are plotted in \Fig{fig:hyperfine}.

\chapter{Derivation of quadrupole GW radiation}
\label{sec:quadrupole}
In this appendix, we demonstrate the derivation of the quadrupolar radiation formula for GW emission, in the limit where the wavelength of the radiation is much larger than the size of the source. Our discussion follows closely that of \cite{Maggiore:2007ulw}.\par
The GW strain outside of a source in the transverse-traceless (TT) gauge is given in \cite{Maggiore:2007ulw},
\begin{equation}
 \label{eq:h_general}
   h^{\rm TT}_{ij}({\bf x},t)=4\Lambda_{ij,lm}(\hat{\bf n})\int \frac{d^3{\bf x}'}{|{\bf x}-{\bf x}'|}T_{lm}({\bf x}',t-|{\bf x-x}'|),
\end{equation}
where $T_{lm}$ is the stress tensor of the source, $\hat{\bf n}$ is the propagation direction of GW, and $\Lambda_{ij,lm}(\hat{\bf n})\equiv P_{il}P_{jm}-\frac{1}{2}P_{ij}P_{lm}$, $i,\,j,\,l,\,m=1,\,2,\,3$, with $P_{ij}(\hat{\bf n})=\delta_{ij}-n_in_j$ the transverse projector. In the far zone limit, $r\equiv|{\bf x}|\gg|{\bf x}'|_{\rm max}$, the strain reduces to,
\begin{equation}
\label{eq:hTT_far_zone}
    h^{\rm TT}_{ij}({\bf x},t)\simeq\frac{4}{r}\Lambda_{ij,lm}(\hat{\bf n})\int d^3{\bf x}'T_{lm}({\bf x}',t-r+\hat{\bf x}\cdot{\bf x}').
\end{equation}
It is convenient to rewrite the above integral in terms of the Fourier transform of the stress tensor,
\begin{equation}
   \label{eq:T_k}
     T_{lm}({\bf x}',t-r+\hat{\bf x}\cdot{\bf x}')=\int \frac{d^4 k}{(2\pi)^4}\tilde{T}_{lm}({\bf k},\omega)e^{-i\omega(t-r+\hat{\bf x}\cdot{\bf x}')+i{\bf k}\cdot {\bf x}'},
\end{equation}
where the wavevector and frequency of the GW satisfy $|{\bf k}|=\omega$.
If $\tilde{T}_{lm}({\bf k},\omega)$ of the source peaks around a characteristic frequency $\omega_c$, with its inverse much larger than the size of the GW source $\lambda=2\pi/\omega_c\gg |{\bf x}'|_{\rm max}$, then it is valid to do the Taylor expansion of the exponent in \Eq{eq:T_k}. 
As we show in \Eq{eqn:peak freq}, the GW wavelength associated with the hyperfine transition is much larger than the size of the GA, $\lambda\simeq \pi/(\Delta m\Omega_{0,{\rm hyp}})\gg r_c$. So, the exponent in \Eq{eq:T_k} takes the form
\begin{equation}
    e^{-i\omega(t-r+\hat{\bf x}\cdot{\bf x}')}= e^{-i\omega(t-r)}[1-i\omega \hat{\bf x}\cdot{\bf x}'+\mathcal{O}(\omega |{\bf x}'|_{\rm max})^2],
\end{equation}
which, in the leading order, is equivalent to rewriting the stress tensor
\begin{equation}
\label{eq:Tlm_far_zone}
    T_{lm}({\bf x}',t-r+\hat{\bf x}\cdot{\bf x}')\simeq T_{lm}({\bf x}',t-r)+(\hat{\bf x}\cdot{\bf x}')\partial_0T_{lm}({\bf x}',t-r).
\end{equation}
In the linearized theory, by neglecting the backreaction of the GW, the energy-momentum tensor $T_{\mu\nu}$ satisfies the conservation equation
\begin{equation}
\label{eq:conservation}
    \partial_\mu T^{\mu\nu}=0, ~~\mu,\nu=0,1,2,3.
\end{equation}
The temporal component of the conservation equation indicates mass conservation, 
\begin{equation}
    \dot{M}=\int_V d^3{\bf x}' \partial_0T^{00}=-\int_V d^3{\bf x}' \partial_iT^{i0}=-\int_{\partial V} dS^i T^{i0}=0, 
\end{equation}
where the boundary $\partial V$ is chosen outside of the source, while the spatial component indicates momentum conservation,
\begin{equation}
    \dot{P}^i= \int_V d^3{\bf x}' \partial_0T^{0i}=-\int_{\partial V} dS^j T^{ji}=0.
\end{equation}
The higher order momenta of $M$ and $P^i$ and their time derivatives can be derived similarly, and the momenta of the stress tensor $S^{ij}$ can be expressed in terms of these quantities, 
\begin{equation}
\label{eq:Sij}
    S^{ij}\equiv \int d^3{\bf x}'T^{ij}=\frac{1}{2}\ddot{M}^{ij},
\end{equation}
where $M^{ij}\equiv \int d^3{\bf x}'{x'}^i{x'}^j T^{00} (t,\vec{x}')$ is the mass quadrupole moment. Therefore, in the leading order, the GW strain is given by combining \Eq{eq:hTT_far_zone}, \Eq{eq:Tlm_far_zone} and \Eq{eq:Sij} and is the result of \Eq{eqn:quadrupole formula h}.

The above derivation shows that the leading contribution to the GW strain is the quadrupole radiation when the characteristic wavelength of the Fourier mode $\tilde{T}_{ij}$ is much larger than the size of the source and energy-momentum conservation is satisfied.


\chapter{Frequency spectrum and stationary phase approximation}
\label{sec:freq spectrum}
In this appendix, we go into more detail about the calculation of the frequency spectrum. It is given by the Fourier transform of the strain $h(t)$:
\begin{equation}
    \tilde{h}_{+,\times}(\omega) = \int dt h_{+,\times}(t) e^{i \omega t},
\label{eqn:fourier h}\end{equation}
Focusing on the plus polarization, 
\begin{equation}
    \tilde{h}_{+}(\omega)  = h_{0} \frac{1+\cos^{2}\iota}{2} \frac{e^{i \omega r }}{2}\int d t \left( e^{i(\omega t - 2 \Delta m \varphi(t))}Q(t) + e^{i(\omega t + 2 \Delta m \varphi(t))}Q^{\ast}(t) \right),
\label{eqn:Ip}\end{equation}
where we have renamed $t_{\rm re} \rightarrow t$.\par
For positive frequencies, the stationary phase approximation can be used to evaluate the above integrals. The approximation is based on the fact that the integrals are dominated at the stationary points, that is, the points where the first derivative of the phase is zero. Since $\dot{\varphi}(t) = \Omega(t)>0$, the first integral does not have a stationary point and the fast oscillations average to zero. The stationary point of the second integral is $t_{+}(\omega) = \frac{\omega - \omega_{\rm c}}{2 |\Delta m| \gamma}$, where we defined $\omega_{\rm c} \equiv 2 |\Delta m| \Omega_{0} = 4 \Omega_{0}$.
 \par
Evaluating the $Q$ factor at this stationary point, Taylor expanding the phase around the it to order $t^{2}$, and calculating the Gaussian integrals, we find
\begin{equation}
    \tilde{h}_{+}(\omega)  = \frac{\sqrt{\pi} h_{0} (1+\cos^{2}\iota)}{4 \sqrt{\gamma |\Delta m|}} Q^{\ast}(t_{+}(\omega))e^{i \Psi_{+}(\omega)}, 
\label{eqn:I factors}\end{equation}
with $\Psi_{+}(\omega) = \omega r + \frac{(\omega - \omega_{\rm c})^{2}}{4 |\Delta m| \gamma }-\frac{\pi}{4}$. Using \Eq{eqn: d1^2 gamma>> 1/dt} and \Eq{eqn: d2 gamma>> 1/dt}, we get
\begin{equation}
    \tilde{h}_{+}(f) =  h_{0} (1+\cos^{2} \iota) \sqrt{\pi} |\Delta m|^{2} i e^{i\Psi_{+}(f)} \frac{\sqrt{z}}{|\Gamma| - i \pi (f - f_{\rm c})} e^{- \pi z} e^{-2 z \tan^{-1}( \frac{\pi(f - f_{\rm c})}{ |\Gamma|})},
\label{eqn:Ip with expo}\end{equation}
where we re-expressed the frequency in terms of $f = \frac{\omega}{2 \pi}$. Similar results hold for $\tilde{h}_{\times}(f)$ that only differs by a phase of $\frac{\pi}{2}$. The peak frequency of $ |\tilde{h}(f)|$ is easily found by taking a derivative of \Eq{eqn:Ip with expo} with respect to $f$ and setting it equal to zero, which yields \Eq{eqn:peak freq}.


\chapter{Towards a relativistic computation}
\label{sec:relativistic}
Since our signal is maximized for rather large values of $\alpha$, it is important to check if the non-relativistic approximation that we have employed throughout this paper holds and identify where it fails. Let us start with the comparison between the relativistic and non-relativistic wavefunctions for different values of $\alpha$. A deviation from the non-relativistic approximation would result in different values for the amplitude $\eta$ and hence different values of $z$. In order to check this effect, we used the code available in \cite{hoof2024gettingblackholesuperradiance,hoof_git} to calculate the energy of the $211$ level and combined this with the analysis outlined in \cite{witte2025steppingsuperradianceconstraintsaxions,Dolan:2007mj} to determine the normalized relativistic wavefunction $\tilde{R} = M^{3/2} R$ as a function of the distance $\tilde{r} = r/M$ from the black hole horizon. In \Fig{fig:relativistic}, we show the relativistic wavefunctions for three different values of $\alpha$ and compare to their non-relativstic counterparts. As it is expected, the largest deviations are observed near the black hole horizon for all three cases, while the results converge at the $\tilde{r} \rightarrow \infty$ limit. In addition, as $\alpha$ increases, the relativistic wavefunction deviates more and more from the non-relativistic one, since the GA is much closer to the black hole horizon. However, these deviations appear to be small and will introduce an order one factor at the most.  

\begin{figure}[h!]
    \centering
    \includegraphics[width=0.7\linewidth]{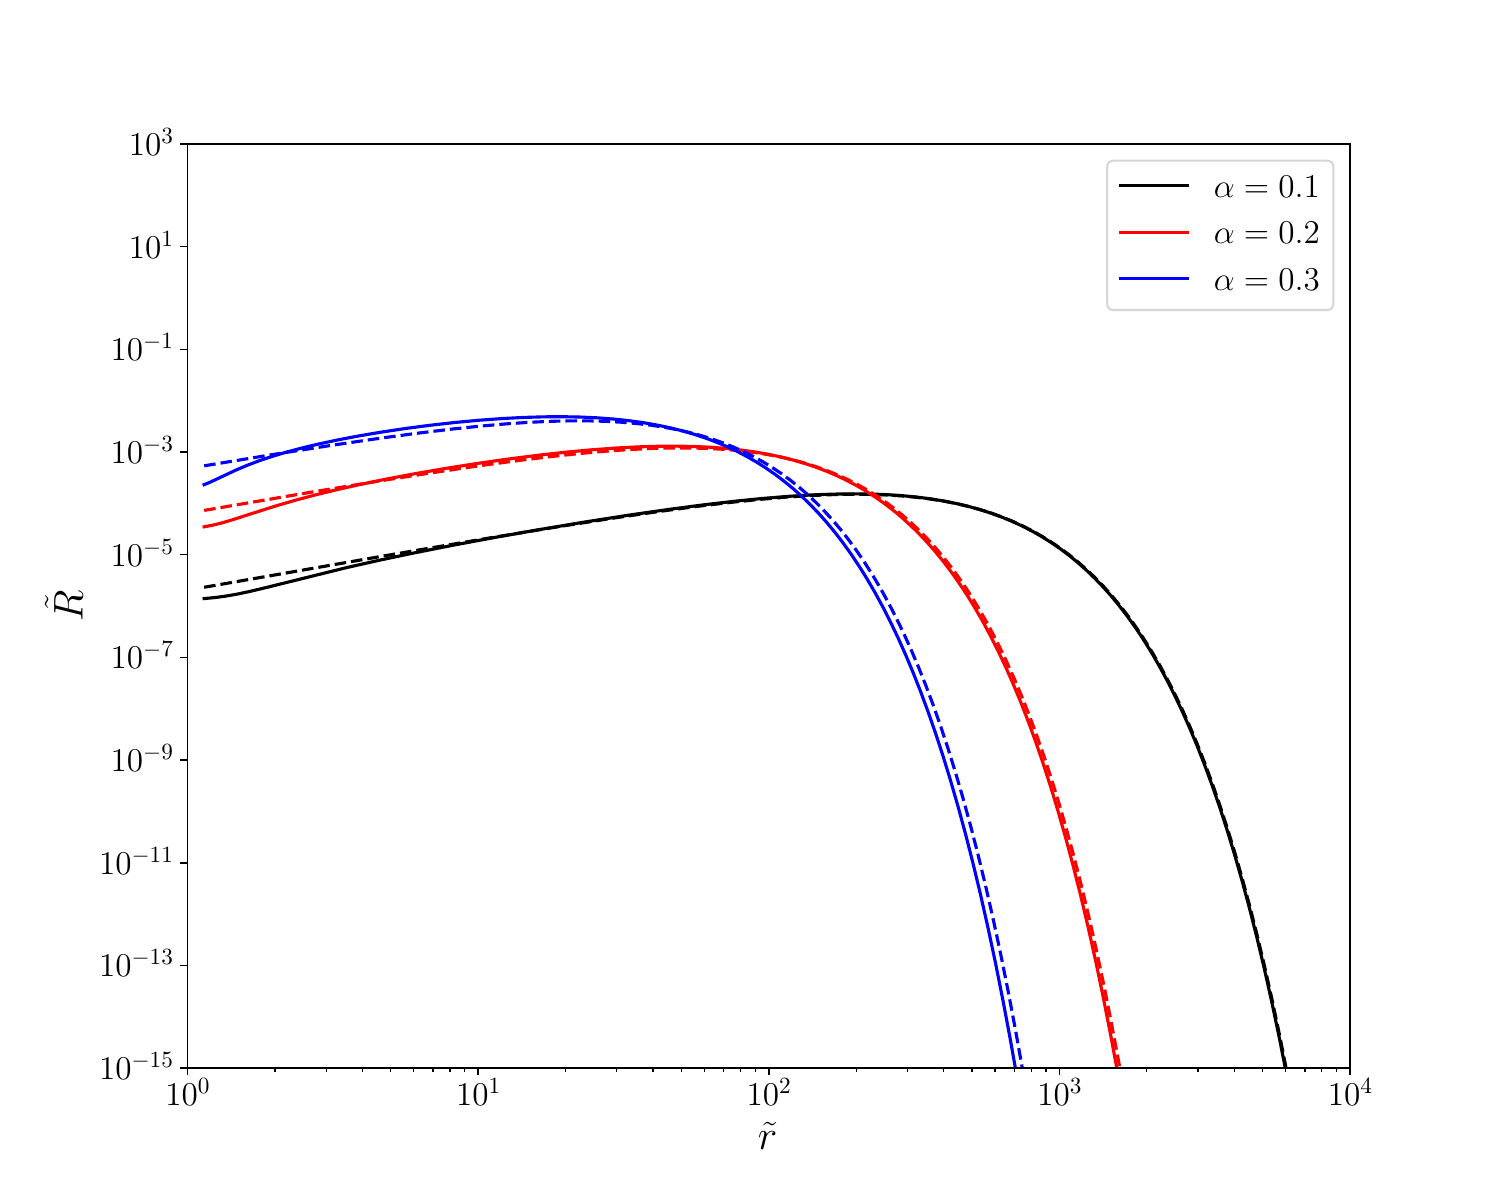}
    \caption[Comparison between relativistic and non-relativistic wavefunctions.]{Comparison between the relativistic wavefunctions (solid lines) with the non-relativistic (dashed lines) for three different values of $\alpha$. We have set $\tilde{a} = 0.99$.\label{fig:relativistic}}
\end{figure} %

\begin{figure}[h!]
\centering
\includegraphics[width=0.7\linewidth]{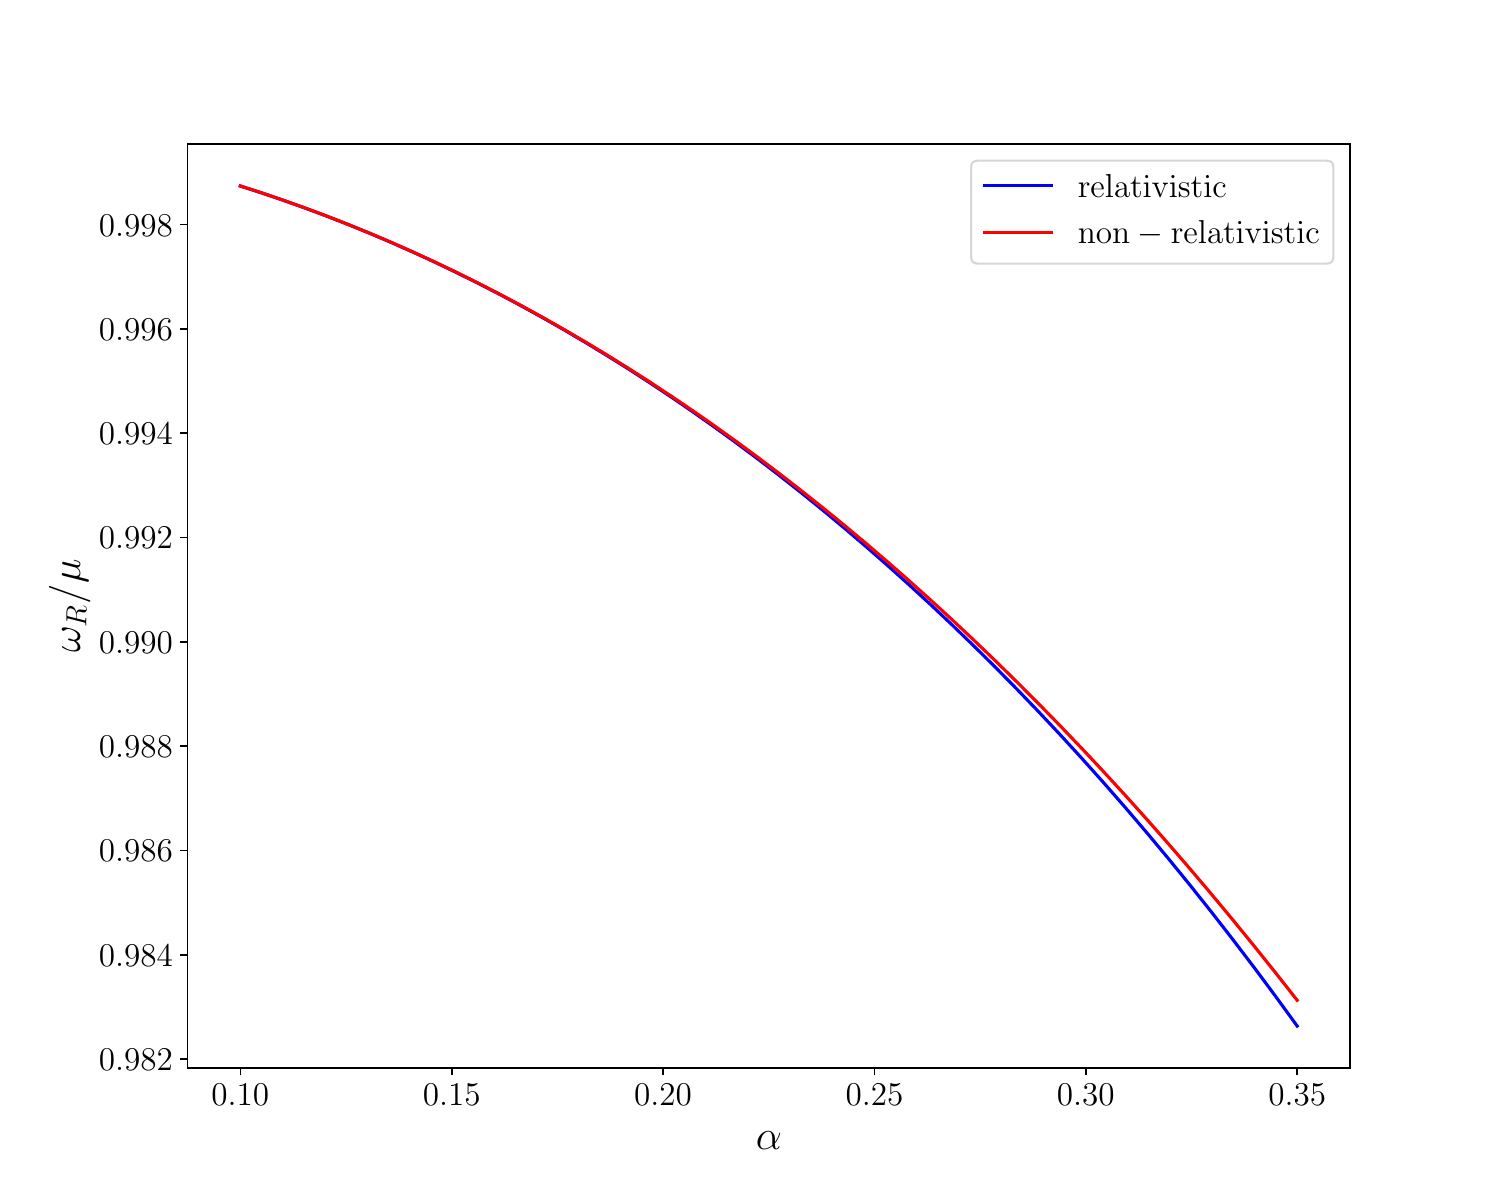}
    \caption[Relativistic and non-relativistic results for the eigenenergy of the 211 state.]{The real energy eigenvalue of the 211 level as a function of $\alpha$, using the relativistic and non-relativistic computations. The black hole's spin is set to $\tilde{a} = 0.99$}
    \label{fig:energy levels}
\end{figure}
\begin{figure}[h!]
\centering
\includegraphics[width=0.7\linewidth]{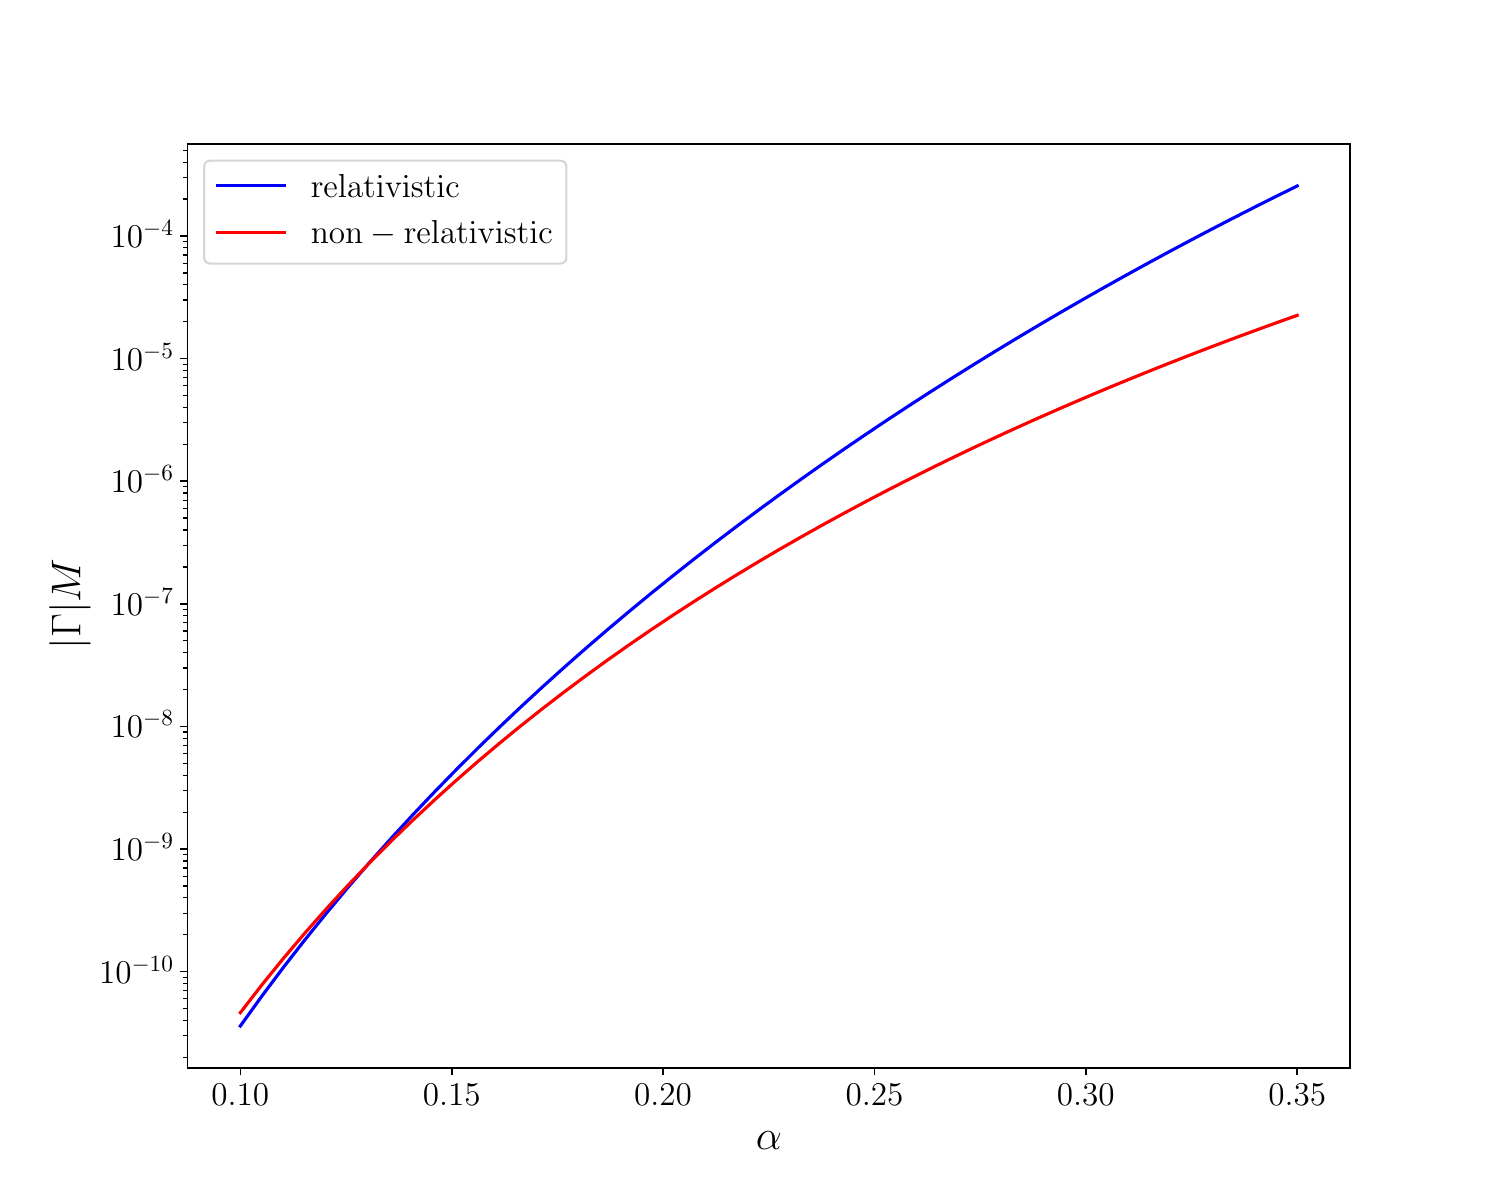}
    \caption[Comparison between the relativistic and non-relativistic calculations of the decay rate.]{The decay rate of the second mode as a function of $\alpha$, comparing the relativistic and non-relativistic computations. The black hole's spin is set to the saturated spin $\tilde{a} = \frac{4\alpha}{1+4\alpha^{2}}$}
    \label{fig:decay rate plot}
\end{figure}
The same behavior shows up for the real part of the energy eigenvalue of the $211$ level, shown in \Fig{fig:energy levels}. The relativistic solution starts to deviate from the non-relativistic one when $\alpha\gtrsim0.3$, but the overall deviation is negligible and should not affect our results. \par
The most important deviation of the relativistic results from the non-relativistic results is in the decay rate of the $|21\text{-}1\rangle$ state, shown in \Fig{fig:decay rate plot}. As it is expected, the non-relativistic computation matches well with the relativistic result in the small $\alpha$ region, $\alpha\lesssim0.15$. However, the two results diverge at most by an order of magnitude at larger $\alpha\le0.35$. This has an important effect on the computation of the SNR, since it inversely proportional to $|\Gamma|$ in \Eq{eqn:SNR mono}. Employing the non-relativistic approximation in this calculation would significantly overestimate the detectability prospects of the signal. 
